# Supplementary material for: PointCrack3D: Crack Detection in Unstructured Environments using a 3D-Point-Cloud-Based Deep Neural Network
Source: arXiv:2111.11615 source file (2021-11-23)
Supplement: Supplementary file 1 [file 8_appendix.tex]

\section*{APPENDIX}

Appendixes should appear before the acknowledgment.
